# Supplementary material for: MDACE: MIMIC Documents Annotated with Code Evidence
Source: arXiv:2307.03859 source file (2023-07-07)
Supplement: Supplementary file 1 [file appendix.tex]

\section{Appendix}
\label{sec:appendix}

\subsection{MIMIC Annotation Guidelines}
\label{sec:guideline}

The task is to annotate MIMIC charts with sufficient code evidence based on the documentations using an open source tool called INCEpTION.

\begin{itemize}
    \item For Inpatient coding, annotate evidence for ICD-10-CM and ICD-10-PCS codes.
    \item For Outpatient coding, annotate evidence for ICD-10-CM and CPT codes (ignoring EM codes).
\end{itemize}

\subsubsection{Install INCEpTION}

Website: \url{https://inception-project.github.io/}

\begin{enumerate}
    \item Install Java from \href{https://java.com/en/download/help/download\_options.html}{Java's website}\footnote{\url{https://java.com/en/download/help/download\_options.html} }
    and choose your OS.
    \item Download INCEpTION 21.1 (executable JAR) from
    \href{https://inception-project.github.io/downloads/}{INCEpTION's repository}\footnote{\url{ https://inception-project.github.io/downloads/}}.
    \item Start INCEpTION by double-clicking the JAR file or using the following command:
    {\small{
    \begin{minted}{bash}
    $ java -jar inception-
    app-webapp-21.1-standalone.jar
    \end{minted}
    }}

    \item Once INCEpTION loads, type \url{localhost:8080} in your web browser and sign in with "admin" for both User ID and Password.
\end{enumerate}

\subsubsection{Create Project}

All documents (OP notes, nursing notes and discharge summary) and codes in an encounter/chart are contained in a folder named with the encounter ID. MIMIC charts come with ICD-9 diagnosis and procedure codes as well as CPT codes, and we used GEM mapping to pair the ICD-10 codes with the ICD-9 codes. Since the mapping is many to many, part of the task is to identify the correct ICD-10 CM/PCS codes based on the documentation.

An INCEpTION project should be created for each chart. Select **Settings** and follow these steps:

1. Copy the zip file to your laptop and unzip:
```
tar xzvf charts.tar.gz
```
2. Click **Create new project** tab, select **Basic annotation (span/relation)**. Name the project "MIMIC-encounterID".
3. Go to **Settings** and then select **Documents**, upload all .txt files in the chart folder.
4. Select **Tagsets**, and then import the .json file in the chart folder. Save the Tagset setting.
5. Go to **Layers**, click **Span** -> **Layer Details** -> **Overlap** and choose **Any**. Then click **Features** -> **Label** and set the following fields:
	- **Tagset**: select Codes-encountID tagset
	- **Editor type**: select **Combo box (mid-size tagsets)**

\subsubsection{Annotate Code Evidence}

Reference the latest coding book to decide whether an I-10 code is supported by the documentation. Code as in real life, once a condition is confirmed and you feel comfortable with a code assignment, annotate the text spans with the code and move on to the next one. You are encouraged to provide multiple evidence for a code pair, as long as it doesn't slow you down too much.

General OP coding guidelines:

- For Profee coding, coders go through all notes and if they see a diagnosis, they will annotate it.
- Usually code external cause codes only with injury codes.
- Follow ICD-10 coding guideline, if there is a definitive diagnosis, coder will not code symptom code, otherwise symptom codes can be coded.
- If notes are duplicated, only code from one of them.

The annotation process includes:

- Leaf through chart documents to find the ones appropriate to code from.
- Highlight best/sufficient text spans as evidence for a code.
- Choose the appropriate ICD-10/ICD-9 code pair or CPT code in the Label box to assign to the highlighted text span.
- If the correct ICD-10 or CPT code is not in the label set, type it in the Label box and assign it to the highlighted text span.
- Try to annotate evidence for all ICD-9 or CPT codes in the label set if there is supporting documentation.
- Do not code EM codes 99201-

To annotate a chart:

1. Go to **Dashboard** and click **Annotation**, select a document to open.
2. Select **Search** for the left panel. You can search any phrase and select the document containing the phrase to annotate.
3. Open the Preferences popup, and set the following (Done once for a project):
	- **Editor**: brat (line-oriented)
	- **Sidebar right**: 30
	- **Page size**: 1000
4. In a document, double click on a word or highlight a text span, and then select a label from the right panel. You can also start typing in the label box and the matching labels will show up.
5. You can navigate through the documents using the icons at the top of the middle panel, and move through the annotations using the arrows in the right panel.

\subsubsection{Export Project}

After you finish annotating a chart, select **Administration** -> **MIMIC-encounterID** -> **Settings** -> **Export**, choose **WebAnno TSV v3.3** format and then **Export the whole project**. Copy the exported zip file to the shared folder.
